# Supplementary material for: 2D Rutherford-Like Scattering in Ballistic Nanodevices
Source: arXiv:1804.02457 source file (2018-04-06)
Supplement: Supplementary file 1 [file Rutherford-like_supplementary-1.pdf]

# Supplementary materials : 2D Rutherford-like scattering in ballistic nanodevices

S. Toussaint,*,† B. Brun-Barrière,† S. Faniel,† L. Desplanque,‡ X. Wallart,‡ V. Bayot,† and B. Hackens*,†

†*Université catholique de Louvain, Institute of Condensed Matter and Nanosciences (IMCN/NAPS), B-1348 Louvain-la-Neuve, Belgium*

‡*Université Lille, CNRS, Centrale Lille, ISEN, Univ. Valenciennes, UMR 8520 - IEMN, F-59000 Lille, France*

E-mail: sebastien.toussaint@uclouvain.be; benoit.hackens@uclouvain.be

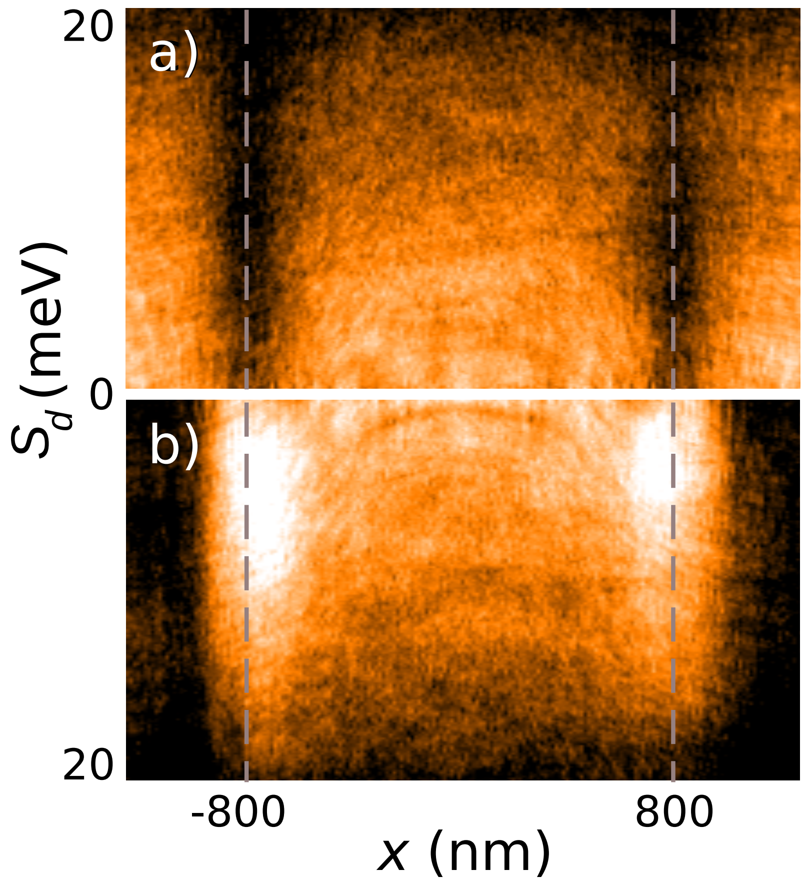


Figure 1: Simulated conductance profiles as the potential perturbation is swept along the black dashed line in Fig. 2a, as a function of $S_d$, with $R_p$ = 150 nm and a) $\varphi_p^{max}$=−0.9 $E_F$ b) $\varphi_p^{max}$=+0.9 $E_F$

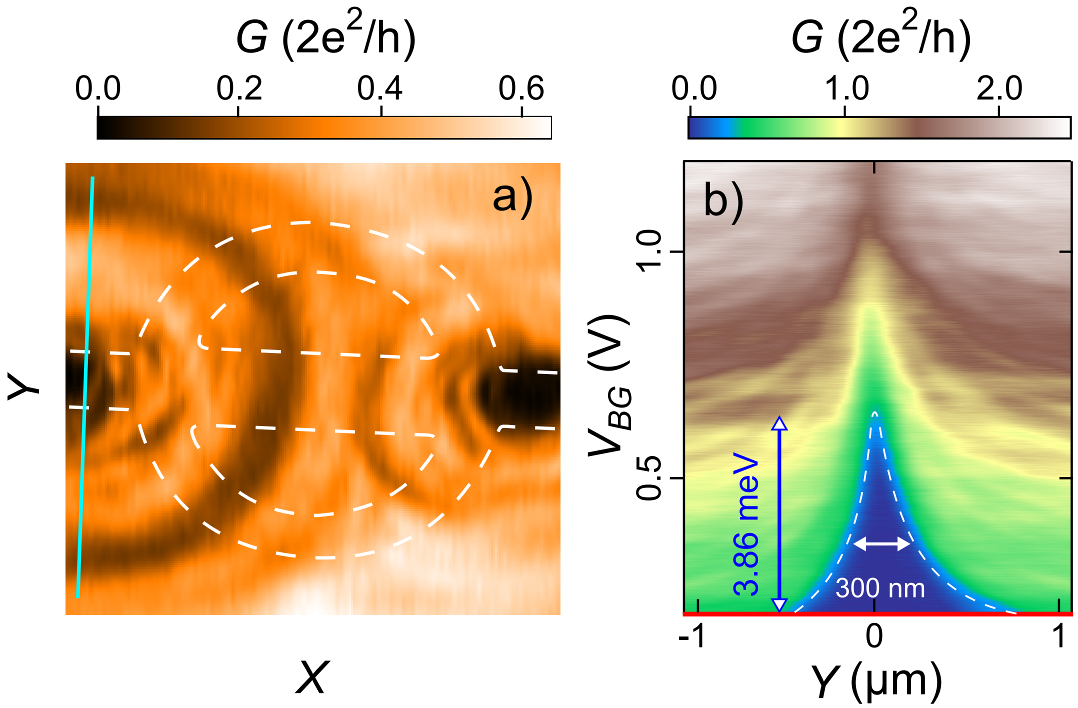


Figure 2: a) Scanning gate microscopy conductance map of a ring-like device fabricated next to the device discussed in the main paper, measured with $V_{BG}$ = 0.3 V, $d_{tip}$ = 80 nm, and $V_{tip}$ = -4 V. White dashed lines in a) delineate the device lithographic layout. The device is close to pinch-off due to the relatively low electron density, which explains the low $G$, and the presence of concentric rings around the narrowest region of the device, corresponding to Coulomb blockade resonances [P. Liu et al., *Physical Review B* 2015, *91*, 075313]. b) Conductance profile measured along the blue line in Fig. S2a), as a function of $V_{BG}$, with $V_{tip}$ = -4 V and $d_{tip}$ = 80 nm. $Y = 0$ corresponds to the center of the entrance channel, which has the same width as the entrance channel of the device discussed in the main text. In the blue region, $G \sim 0$ and the entrance channel is depleted. The edges of this region (dashed white line) correspond to the shape of the tip-induced electrostatic potential, as experienced by electrons confined in the entrance lead. Fitting a lorentzian function to this region yields an amplitude $\Delta V_{BG}$= 0.36 V and full-width at half maximum $\sim$ 300 nm. Thanks to measurements of the electron density in the 2DEG as a function of $V_{BG}$, one can extract a lever-arm of 10.6 meV/V for the back gate, which allows to convert $\Delta V_{BG}$ in $\varphi_p^{max}$= 3.86 meV (as indicated on the figure). To calculate $\varphi_p^{max}$ for other values of $d_{tip}$ and $V_{tip}$, we assume that $\varphi_p^{max}$ scales quadratically with $d_{tip}$, and linearly with $V_{tip}$.

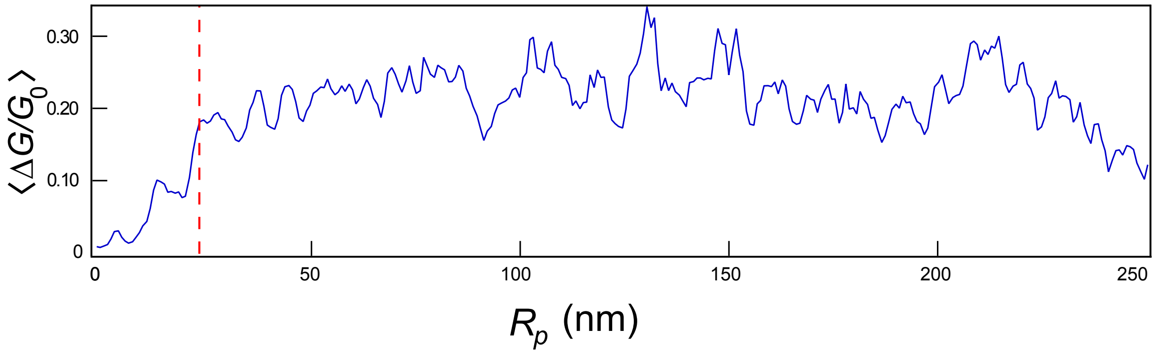


Figure 3: Average of two profiles of $\Delta G/G_0$, measured along the two vertical dashed lines in Fig. 5c, as $R_p$ is varied. The red vertical dashed line corresponds to the Fermi wavelength.

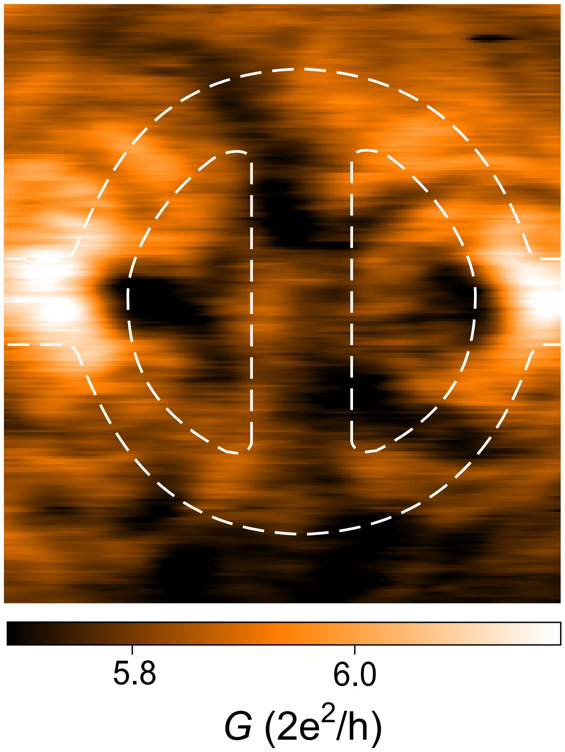


Figure 4: Same conductance map as Fig. 4c), with an enhanced contrast. Circles of reduced conductance are observed around the T-junctions on both sides of the device. These features are reminescent of the Coulomb blockade concentric circles observed around quantum dots forming when the disorder potential fluctuations are raised locally at the Fermi level by the gating action of the tip in lower density structures [P. Liu et al., *Physical Review B* 2015, *91*, 075313]. We speculate that the similar iso-conductance circles observed here, but with a reduced conductance and for a positive gate voltage, may be explained by the presence of local minima in the confinement potential at the edges of the device. Such minima could then be shifted below the Fermi level by a positive tip voltage and become active as quantum dots tunnel-coupled to the transmitted channels.
